# Supplementary material for: Surface acoustic wave driven acoustic spin splitter in d-wave altermagnetic thin films
Source: arXiv:2502.18007 ancillary file (2026-03-25)
Supplement: Supplementary file 1 [file SM.pdf]

# Supplementary Material

## Surface acoustic wave driven spin splitter currents in $d$ -wave altermagnets

Pieter M. Gunnink,<sup>\*</sup> Jairo Sinova, and Alexander Mook

*Institute of Physics, Johannes Gutenberg-University Mainz, Staudingerweg 7, Mainz 55128, Germany*

(Dated: February 25, 2025)

In this supplementary material we derive the main formalism used to obtain the results in the main text. We first consider the general problem of the second order electron response to a surface acoustic wave in a metallic thin film in Section I, which we subsequently apply to a metallic altermagnet in Section II. Next, we use these results to obtain the second order *magnon* response in Section III, which follows much of the same formalism, except the electric field is replaced by a deformation. We apply this to an insulating altermagnet in Section IV to derive the magnon strain coupling in Section V. These results conclude the main formalism of our work.

In the second part of the supplementary material we provide additional details regarding the detection of the transverse spin current (Section VI) and the Bleustein-Gulyaev surface acoustic wave (Section VII). We also discuss why we can ignore out-of-plane electric fields and deformations in Section VIII, and we give additional results discussing the thickness dependency in Section IX.

### Contents

|                                                                              |    |
|------------------------------------------------------------------------------|----|
| I. Electron response to a surface acoustic wave                              | 1  |
| A. First order response                                                      | 2  |
| B. Second order response                                                     | 4  |
| C. Adiabatic limit                                                           | 4  |
| II. Metallic altermagnet                                                     | 5  |
| A. Parameters used for RuO <sub>2</sub>                                      | 6  |
| III. Second order magnon response to a surface acoustic wave                 | 7  |
| IV. Insulating altermagnet                                                   | 8  |
| A. Parameters used in the main text                                          | 10 |
| V. Magnon strain coupling                                                    | 10 |
| VI. Detecting the transverse spin current with a heavy metal                 | 12 |
| VII. Details of a Bleustein-Gulyaev surface acoustic wave                    | 13 |
| VIII. Effect of the electric field and deformation force along the $z$ -axis | 13 |
| IX. Thickness dependency                                                     | 14 |
| References                                                                   | 14 |

### I. Electron response to a surface acoustic wave

We first consider a metallic thin film, where the SAW travelling in the piezoelectric substrate generates a piezoelectric field, which couples to the electrons. The coupling to the magnons then follows analogously, which we will discuss in more detail in Section III.

---

<sup>\*</sup> [pgunnink@uni-mainz.de](mailto:pgunnink@uni-mainz.de)

The dynamics of the electron distribution function  $f^\sigma$  of spin  $\sigma$  are described by the Boltzmann equation

$$\partial_t f^\sigma + \mathbf{v}_\mathbf{k}^\sigma \cdot \nabla_\mathbf{r} f^\sigma + \frac{e}{\hbar} [\mathbf{E}(\mathbf{r}, t) + \mathbf{E}_i(\mathbf{r}, t)] \cdot \nabla_\mathbf{k} f^\sigma = -\frac{f^\sigma - \langle f^\sigma \rangle}{\tau}, \quad (1)$$

where  $\mathbf{v}_\mathbf{k}^\sigma \equiv \nabla_\mathbf{k} \omega_\mathbf{k}^\sigma$  is the group velocity of electrons with spin  $\sigma$  described by the dispersion  $\hbar \omega_\mathbf{k}^\sigma$ ,  $\langle f^\sigma \rangle$  is the equilibrium distribution function of electrons with spin  $\sigma$  and  $\tau$  is the relaxation time. Here we have made the relaxation time approximation [1] and have assumed that the two spin branches are independent, i.e., there is no spin-orbit coupling which allows for scattering between the two branches.

The electric field  $\mathbf{E}(\mathbf{r}, t)$  is generated by a Bleustein-Gulyaev SAW [2, 3] travelling in the adjacent piezoelectric,

$$\mathbf{E}(\mathbf{r}, t) = \mathbf{E} e^{i\mathbf{q} \cdot \mathbf{r} - i\omega t} / 2 + \text{c.c.}, \quad (2)$$

where the electric field contains a component orientated along the wavevector,  $\mathbf{E} \parallel \mathbf{q}$ , as well as an out-of-plane component,  $\mathbf{E} \parallel \mathbf{q}$ , such that  $\mathbf{E} = E_\parallel \hat{\mathbf{q}} + E_z \hat{\mathbf{z}}$ . The out-of-plane component will however not play an important role in the acoustically driven spin current, and will be disregarded from here on. We discuss this in more detail in Section VIII. Furthermore, there is an induced electric field,  $\mathbf{E}_i$ , induced by the fluctuations of the electron density. Finally,  $e$  is the electron charge and  $\hbar$  is the reduced Planck constant.

In addition, there will also be a force on the electrons due to the deformation of the lattice. We expect however that the force from the electric field will be much stronger [4], and will therefore disregard the effects of the deformation on the electron dynamics.

Since the applied electric field acts as a perturbation of the equilibrium state described by  $\langle f^\sigma \rangle$ , we expand the distribution function in  $|\mathbf{E}|$ . However, since the applied electric field is oscillating in time, there will be only an AC response in first order response [since the time-average of the force, i.e., of  $\mathbf{E}(\mathbf{r}, t)$ , is zero]. Up to second order in the electric field however, there will be a DC and AC response. Following [5], we therefore expand the distribution function and electron densities up to second order,

$$n^\sigma(\mathbf{r}, t) = n^\sigma + n_1^\sigma(\mathbf{r}, t) + n_2^\sigma(\mathbf{r}, t), \quad (3)$$

$$f^\sigma(\mathbf{r}, t) = f_0^\sigma + f_1^\sigma(\mathbf{r}, t) + f_2^\sigma(\mathbf{r}, t), \quad (4)$$

$$\langle f^\sigma(\mathbf{r}, t) \rangle = f_0^\sigma + [n_1^\sigma(\mathbf{r}, t) + n_2^\sigma(\mathbf{r}, t)] \frac{\partial f_0^\sigma}{\partial n^\sigma}, \quad (5)$$

where the numerical subscripts denote the power in  $|\mathbf{E}|$  and

$$f_0^\sigma = \left[ \exp \left( \frac{\epsilon_\mathbf{k}^\sigma - \mu(n^\sigma)}{k_B T} \right) + 1 \right]^{-1} \quad (6)$$

is the equilibrium Fermi-Dirac distribution function, which depends on the electron density  $n^\sigma$  through the chemical potential  $\mu$ . Here  $k_B$  is the Boltzmann constant and  $T$  is the electron temperature. We furthermore disregard any heating effects and will therefore assume the temperature to be constant.

### A. First order response

Now collecting the leading order contributions to the Boltzmann equation we find that the first-order response can be written as

$$\left( \frac{1}{\tau} + i\mathbf{v}_\mathbf{k}^\sigma \cdot \mathbf{q} - i\omega \right) f_1^\sigma = -\frac{1}{\hbar} (e\mathbf{E} + e\mathbf{E}_i) \cdot \nabla_\mathbf{k} f_0^\sigma + \frac{n_1^\sigma}{\tau} \frac{\partial f_0^\sigma}{\partial n^\sigma}. \quad (7)$$

We now solve this for  $f_1^\sigma$  to obtain

$$f_1^\sigma = \frac{-\tau(e\mathbf{E} + e\mathbf{E}_i) \cdot \mathbf{v}_\mathbf{k}^\sigma (\partial_{\epsilon_\mathbf{k}} f_0^\sigma) + n_1^\sigma \frac{\partial f_0^\sigma}{\partial n^\sigma}}{1 - i\mathbf{v}_\mathbf{k}^\sigma \cdot \mathbf{q}}, \quad (8)$$

where

$$\mathbf{v}_\mathbf{k}^\sigma \equiv \tau(\omega - \mathbf{v}_\mathbf{k}^\sigma \cdot \mathbf{q}). \quad (9)$$

In addition, the induced movement of the electrons will also create an induced electric field  $\mathbf{E}_i$  [6]. Assuming that  $qd \ll 1$ , with  $d$  the thickness of the film, we can treat this in the two-dimensional limit [7]. The induced field can then be found from Maxwell's equation

$$\nabla \cdot \mathbf{D}_i = \rho, \quad (10)$$

where  $\mathbf{D}_i = \epsilon_0 \epsilon \mathbf{E}_i$ , with  $\epsilon_0$  the vacuum permittivity and  $\epsilon$  the average dielectric function of the surrounding environment, i.e.,  $\epsilon \equiv (\epsilon_{PZ} + 1)/2$  of the piezoelectric below and the vacuum above. The charge density is  $\rho = e[N(\mathbf{r}, t) - \sum_{\sigma} n^{\sigma}(\mathbf{r}, t)]$ , with  $N(\mathbf{r}, t)$  the background charge.

Expanding  $n^{\sigma}(\mathbf{r}, t)$  up to first order in  $n_1$  and Fourier transforming we can directly solve for

$$\mathbf{E}_i = -i \sum_{\sigma} \frac{ed}{\epsilon_0(1 + \epsilon)} n_1^{\sigma} \hat{\mathbf{q}}. \quad (11)$$

We now need to determine  $n_1^{\sigma}$ , which is done by requiring charge conservation, i.e.,

$$\partial_t n_1^{\sigma} + \nabla \cdot \mathbf{j}_1^{\sigma} = 0, \quad (12)$$

where

$$\mathbf{j}_1^{\sigma} = \int \frac{d\mathbf{k}}{(2\pi)^d} \mathbf{v}_{\mathbf{k}}^{\sigma} f_1^{\sigma} \quad (13)$$

is the first order particle current density. Inserting  $f_1^{\sigma}$  from Eq. (8) into Eq. (13) we obtain

$$\mathbf{j}_1^{\sigma} = \sum_{\sigma} \int \frac{d\mathbf{k}}{(2\pi)^d} \frac{\mathbf{v}_{\mathbf{k}}^{\sigma}}{1 - i\nu_{\mathbf{k}\sigma}} \left[ -n_1^{\sigma} \frac{\partial n^{\sigma}}{\partial \mu} + i(n_1^{\uparrow} + n_1^{\downarrow}) \frac{de^2 \tau}{\epsilon_0 q(1 + \epsilon)} \mathbf{q} \cdot \mathbf{v}_{\mathbf{k}}^{\sigma} \right] \frac{\partial f_0^{\sigma}}{\partial \epsilon_{\mathbf{k}\sigma}} - \frac{e\tau}{\hbar} \int \frac{d\mathbf{k}}{(2\pi)^d} \frac{\mathbf{v}_{\mathbf{k}\sigma}}{1 - i\nu_{\mathbf{k}\sigma}} \frac{\partial f_0}{\partial \epsilon_{\mathbf{k}\sigma}} (\mathbf{v}_{\mathbf{k}\sigma} \cdot \mathbf{E}). \quad (14)$$

Following Kittel and Fong [8], we now identify the conductivity tensor

$$\sigma_{\alpha\beta}^{\sigma} = -e^2 \tau \int \frac{d\mathbf{k}}{(2\pi)^d} \frac{v_{\mathbf{k}\alpha}^{\sigma} v_{\mathbf{k}\beta}^{\sigma}}{1 - i\nu_{\mathbf{k}\sigma}} \frac{\partial f_0^{\sigma}}{\partial \epsilon_{\mathbf{k}\sigma}} \quad (15)$$

and the diffusion vector

$$R_{\alpha}^{\sigma} = -\frac{\partial \mu}{\partial n} \int \frac{d\mathbf{k}}{(2\pi)^d} \frac{v_{\mathbf{k}\alpha}^{\sigma}}{1 - i\nu_{\mathbf{k}\sigma}} \frac{\partial f_0^{\sigma}}{\partial \epsilon_{\mathbf{k}\sigma}}. \quad (16)$$

Using these definitions, we now write Eq. (14) as

$$j_{1;\alpha}^{\sigma} = n_1^{\sigma} R_{\alpha}^{\sigma} + \sum_{\beta} \sigma_{\alpha\beta}^{\sigma} \left( E^{\beta} / \hbar e - i(n_1^{\uparrow} + n_1^{\downarrow}) \frac{dq_{\beta}}{q\epsilon_0(1 + \epsilon)} \right) \quad (17)$$

and insert it into the continuity equation (12) to solve for  $n_1^{\sigma}$  as

$$n_1^{\sigma} = \frac{1}{e} \sum_{\alpha\beta} \frac{q^{\alpha} \sigma_{\alpha\beta}^{\sigma} E^{\beta}}{(\omega - q_{\alpha} R_{\alpha}^0)(1 + ig(\mathbf{q}, \omega))}; \quad g(\mathbf{q}, \omega) \equiv \sum_{\alpha\beta} \frac{q^{\alpha} q^{\beta} v_{\alpha\beta}^*}{q(\omega - q_{\alpha} R_{\alpha}^0)}, \quad (18)$$

where we have neglected the  $\sigma$ -dependency of the diffusion vector  $R_{\alpha}$ , defining  $R_{\alpha}^0 \equiv \frac{1}{2} \sum_{\sigma} R_{\alpha}^{\sigma}$ . Here  $1 + ig(\mathbf{q}, \omega)$  contains the corrections due to the induced field, and is thus related to the dielectric function. Additionally,

$$v_{\alpha\beta}^* = \frac{d\sigma_{\alpha\beta}^0}{\epsilon_0(1 + \epsilon)} \quad (19)$$

is the velocity of charge spreading, where we have defined  $\sigma_{\alpha\beta}^0 \equiv \sum_{\sigma} \sigma_{\alpha\beta}^{\sigma}$ .

## B. Second order response

For the second order, we first focus on the DC component and thus require that  $\partial_t f_2^\sigma = 0$ . We obtain by expanding the Boltzmann equation (1) up the second order,

$$\frac{e}{4\hbar}(\mathbf{E} + \mathbf{E}_i + \mathbf{E}^* + \mathbf{E}_i^*) \cdot \nabla_{\mathbf{k}}(f_1^\sigma + f_1^{\sigma*}) = -\frac{1}{\tau} \left( f_2^\sigma - \bar{n}_2^\sigma \frac{\partial f_0^\sigma}{\partial n} - \frac{n_1^\sigma n_1^{\sigma*}}{4} \frac{\partial^2 f_0^\sigma}{\partial n^2} \right), \quad (20)$$

where  $\bar{n}_2^\sigma$  indicates time-averaging. For the stationary part, i.e. the DC component, we drop terms  $\propto e^{2i\omega t}$ . Furthermore, the second and third terms on the right-hand side of Eq. (20) are even functions of  $\mathbf{k}$  and only enter in the final result combined with the group velocity  $\mathbf{v}_{\mathbf{k}}^\sigma$ . Therefore, once integrated over  $\mathbf{k}$  they will not contribute and we can disregard them from here on.

We thus obtain

$$\frac{e}{4\hbar}(\mathbf{E} + \mathbf{E}_i) \cdot \nabla_{\mathbf{k}} f_1^{\sigma*} + \frac{e}{4\hbar}(\mathbf{E}^* + \mathbf{E}_i^*) \cdot \nabla_{\mathbf{k}} f_1^\sigma = -\frac{f_2^\sigma}{\tau}. \quad (21)$$

We can now directly solve for

$$f_2^\sigma = -\frac{\tau e}{4\hbar}(\mathbf{E} + \mathbf{E}_i) \cdot \nabla_{\mathbf{k}} f_1^{\sigma*} + \frac{\tau e}{4\hbar}(\mathbf{E}^* + \mathbf{E}_i^*) \cdot \nabla_{\mathbf{k}} f_1^\sigma \quad (22)$$

$$= -\frac{\tau e}{2\hbar} \text{Re}[(\mathbf{E} + \mathbf{E}_i) \cdot \nabla_{\mathbf{k}} f_1^{\sigma*}] \quad (23)$$

and obtain the particle current through the relation

$$\mathbf{j}_2^\sigma = \int \frac{d\mathbf{k}}{(2\pi)^d} \mathbf{v}_{\mathbf{k}}^\sigma f_2^\sigma \quad (24)$$

as

$$\mathbf{j}_2^\sigma = -\frac{\tau}{2} \text{Re} \int \frac{d\mathbf{k}}{(2\pi)^d} \mathbf{v}_{\mathbf{k}}^\sigma (e\mathbf{E}^*/\hbar + e\mathbf{E}_i^*/\hbar) \cdot \nabla_{\mathbf{k}} f_1^\sigma. \quad (25)$$

Integrating by parts we obtain

$$\mathbf{j}_2^\sigma = \frac{\tau}{2} \sum_{\beta} \text{Re} \left[ (eE_{\beta}^*/\hbar + eE_{i\beta}^*/\hbar) \int \frac{d\mathbf{k}}{(2\pi)^d} \frac{\partial \mathbf{v}_{\mathbf{k}\alpha}^\sigma}{\partial k_{\beta}} f_1^\sigma \right]. \quad (26)$$

This concludes the second order DC response, which can be directly evaluated if a dispersion relation is given.

In addition to the second order DC response we have derived above, there is also a second harmonic response that contains terms  $e^{i2\omega t}$ . This can be solved for by collecting all terms  $\propto e^{2i\omega t}$  in Eq. (20), such that we obtain

$$f_{(2\omega)}^\sigma = -\frac{\tau e}{4\hbar(1-2i\omega\tau)}(\mathbf{E} + \mathbf{E}_i) \cdot \nabla_{\mathbf{k}} f_1^\sigma + \frac{\tau e}{4\hbar(1-2i\omega\tau)}(\mathbf{E}^* + \mathbf{E}_i^*) \cdot \nabla_{\mathbf{k}} f_1^{\sigma*} \quad (27)$$

$$= -\frac{\tau e}{2\hbar(1-2i\omega\tau)} \text{Re}[(\mathbf{E} + \mathbf{E}_i) \cdot \nabla_{\mathbf{k}} f_1^\sigma] \quad (28)$$

where we have neglected  $n_2$ , because it will give contributions of order  $\tau^2$ . Integrating by parts we obtain

$$\mathbf{j}_{(2\omega)}^\sigma = \frac{1}{2} \frac{\tau}{(1-2i\omega\tau)} \sum_{\beta} \text{Re} \left[ (eE_{\beta}/\hbar + eE_{i\beta}/\hbar) \int \frac{d\mathbf{k}}{(2\pi)^d} \frac{\partial \mathbf{v}_{\mathbf{k}\alpha}^\sigma}{\partial k_{\beta}} f_1^\sigma \right]. \quad (29)$$

## C. Adiabatic limit

In what follows, we assume the adiabatic limit, i.e.,  $\omega\tau \ll 1$  and  $\mathbf{q} \cdot \mathbf{v}_{\mathbf{k}}^\sigma$  such that  $v_{\mathbf{k}} \ll 1$ . This can reasonably be achieved given the frequency and velocity mismatch between typical SAWs and (thermal) electrons.<sup>1</sup> We then find from Eq. (8)

$$f_1^\sigma = -\tau(e\mathbf{E} + e\mathbf{E}_i) \cdot \mathbf{v}_{\mathbf{k}}^\sigma (\partial_{\epsilon_{\mathbf{k}}} f_0^\sigma) + n_1^\sigma \frac{\partial f_0^\sigma}{\partial n}. \quad (30)$$

<sup>1</sup> Explicitly, for the parameters used in this work we have that  $\omega\tau \approx 10^{-6}$  and  $\tau\mathbf{q} \cdot \mathbf{v}_{\mathbf{k}}^\sigma \approx 10^{-4}$ , for  $\omega/2\pi = 0.5$  GHz.

We can now find the first order current at frequency  $\omega$  from Eq. (17) as

$$j_{(\omega)\alpha}^\sigma = \frac{\sigma_{\alpha\alpha}^\sigma E}{e} \left( \frac{1}{\hbar} - i \frac{\sigma_{\alpha\alpha}^0 \zeta_\sigma}{1 + ig^0(\mathbf{q}, \omega)} \right), \quad (31)$$

where we note that the typical  $1/(1 - i\omega\tau)$  term has already been absorbed in the definition of the conductivity  $\sigma^0$ , see Eq. (15).

We can furthermore insert the electron density  $n_q^\sigma$ , Eq. (18), in the induced field, Eq. (11), to find

$$\mathbf{E}_i = -ig(\mathbf{q}, \omega) \frac{E}{1 + ig(\mathbf{q}, \omega)} \hat{\mathbf{q}}, \quad (32)$$

where we made use of the fact that the induced field, electric field and  $\mathbf{q}$  are parallel to each other.

Inserting Eqs. (30) and (32) into Eq. (26) we find in DC response a drift current,

$$j_{\text{drift};(0)\alpha}^\sigma = -\frac{\tau^2}{2} \sum_\beta \text{Re} \left[ (eE_\beta^* + eE_{i\beta}^*)(eE_\beta + eE_{i\beta}) \int \frac{d\mathbf{k}}{(2\pi)^d} v_{\mathbf{k}\beta}^\sigma \frac{\partial v_{\mathbf{k}\alpha}^\sigma}{\partial k_\beta} \frac{\partial f_0^\sigma}{\partial \epsilon_{\mathbf{k}}} \right], \quad (33)$$

and a diffusion current,

$$j_{\text{diff};(0)\alpha}^\sigma = -\frac{1}{\hbar} \sum_\beta \int \frac{d\mathbf{k}}{(2\pi)^d} \frac{\partial \mu}{\partial n} \frac{\tau}{2e^2} \text{Re} \left[ \frac{(eE_\beta^* + eE_{i\beta}^*) q^\beta \sigma_{\beta\beta}^\sigma eE^\beta}{(\omega - \mathbf{q} \cdot \mathbf{R})(1 + ig(\mathbf{q}, \omega))} \frac{\partial v_{\mathbf{k}\alpha}^\sigma}{\partial k_\beta} \frac{\partial f_0^\sigma}{\partial \epsilon_{\mathbf{k}}} \right]. \quad (34)$$

Importantly, the drift current vanishes in the limit of  $v_{\mathbf{k}}^\sigma \ll 1$ , since  $v_{\mathbf{k}\beta}^\sigma$  is an odd function of momentum. In what follows, we can thus neglect the drift current and focus on the diffusion current, which is given by

$$j_{(0)\alpha}^\sigma = -\frac{\tau}{2\hbar} \frac{\partial \mu}{\partial n} \frac{q \sigma_0^\sigma}{\omega} \frac{|E|^2}{1 + \zeta^2} \int \frac{d\mathbf{k}}{(2\pi)^d} \frac{\partial v_{\mathbf{k}\alpha}^\sigma}{\partial k_\beta} \frac{\partial f_0^\sigma}{\partial \epsilon_{\mathbf{k}}}, \quad (35)$$

where  $\beta$  is the direction of the SAW. Here we have defined the dimensionless parameter  $\zeta \equiv v^* q / \omega$ , which measure the screening of the piezoelectric field by charge spreading, and we have neglected the diffusive contribution proportional to  $\mathbf{q} \cdot \mathbf{R} / \omega$ .<sup>2</sup>

Analogously, we obtain for the second harmonic response

$$j_{(2\omega)\alpha}^\sigma = -\frac{\tau}{2\hbar} \frac{\partial \mu}{\partial n} \frac{q \sigma_0^\sigma}{\omega} \frac{|E|^2 (1 - \zeta^2)}{(1 + \zeta^2)^2} \int \frac{d\mathbf{k}}{(2\pi)^d} \frac{\partial v_{\mathbf{k}\alpha}^\sigma}{\partial k_\beta} \frac{\partial f_0^\sigma}{\partial \epsilon_{\mathbf{k}}}, \quad (36)$$

where we have again used that  $\omega\tau \ll 1$ . Alternatively, we can write

$$j_{(2\omega)\alpha}^\sigma = \frac{1 - \zeta^2}{1 + \zeta^2} j_{(0)\alpha}^\sigma. \quad (37)$$

## II. Metallic altermagnet

We consider a metallic altermagnet orientated such that the long-wavelength electron dynamics can be described by

$$\epsilon_{\mathbf{k}}^\sigma = \frac{\hbar^2 k^2}{2m} + \sigma \alpha_e k_x k_z. \quad (38)$$

We can now explicitly perform the integration over  $\mathbf{k}$  in Eqs. (35) and (36). As discussed in the main text, we required the spin current along the  $z$ -axis, whilst rotating the propagating of the SAW in the plane. We perform a rotation of the crystallographic axis to a frame where the SAW lies along  $\hat{\mathbf{x}}$ , such that we have

$$\mathbf{k} \rightarrow \mathcal{R}^{-1} \mathbf{k}, \quad (39)$$

where

$$\mathcal{R} = \begin{pmatrix} \cos \theta & -\sin \theta & 0 \\ \sin \theta & \cos \theta & 0 \\ 0 & 0 & 1 \end{pmatrix}. \quad (40)$$

<sup>2</sup> For the parameters used in the main text and a SAW frequency of  $\omega/2\pi = 0.5$  GHz, we have that  $\mathbf{q} \cdot \mathbf{R} / \omega \approx 10^{-1}$ .

We obtain

$$\epsilon_{\mathbf{k}}^{\sigma} = \frac{\hbar^2 k^2}{2m} + \sigma \alpha_e k_z (k_x \cos \theta + k_y \sin \theta). \quad (41)$$

Our interest is in the transverse spin current, i.e.,  $(\mathbf{j}^{\uparrow} - \mathbf{j}^{\downarrow}) \cdot \hat{\mathbf{z}}$ . We thus evaluate the  $z$  component of the final current response in Eq. (35) by noting that

$$\int \frac{d\mathbf{k}}{(2\pi)^d} \frac{\hat{\mathbf{z}} \cdot \partial(\mathbf{v}_{\mathbf{k}}^{\uparrow} - \mathbf{v}_{\mathbf{k}}^{\downarrow})}{\partial k_x} \frac{\partial f_0^{\sigma}}{\partial \epsilon_{\mathbf{k}}} = \hbar^{-1} \sigma \alpha_e \cos \theta \int \frac{d\mathbf{k}}{(2\pi)^d} \frac{\partial f_0^{\sigma}}{\partial \epsilon_{\mathbf{k}}}, \quad (42)$$

where we have only kept the asymmetric in  $\sigma$  contributions.

Additionally, the spin splitting will always be the result of the altermagnetic spin splitting and thus be proportional to  $\alpha_e$ , for which typically holds  $\alpha_e < \hbar^2/2m$ . We therefore expand up to first order in  $\alpha_e$ . Since the spin current along  $z$  will always be proportional to  $\alpha_e$  because of Eq. (42), this expansion corresponds to setting  $\alpha_e = 0$  in all other expressions. We can thus approximate

$$\sigma_{xx}^{\sigma} \approx \sigma_0 = \frac{ne^2\tau}{m^*} \quad (43)$$

through the Drude approximation [9] and (at zero temperature)

$$\int \frac{d\mathbf{k}}{(2\pi)^d} \frac{\partial f_0^{\sigma}}{\partial \epsilon_{\mathbf{k}}} \approx D_{\alpha=0}(\epsilon_F), \quad (44)$$

where  $D_{\alpha=0}(\epsilon_F) = \int \frac{d\mathbf{k}}{(2\pi)^d} \delta(\epsilon_F - \hbar k^2/2m)$  is the spin-independent density of states at the Fermi level. Additionally,

$$\frac{\partial \mu}{\partial n} \approx -\frac{1}{D_{\alpha=0}(\epsilon_F)}. \quad (45)$$

Furthermore,

$$R = -i \frac{q}{e^2} \frac{\partial \mu}{\partial n} \sigma_0. \quad (46)$$

We can now directly write down the induced spin current along the  $\hat{\mathbf{z}}$  direction,<sup>3</sup>

$$j_s^z \equiv j_y^{\uparrow} - j_y^{\downarrow} = -e \frac{\tau}{\hbar^2} \frac{q\sigma^0}{\omega} \frac{|E|^2}{1 + \zeta^2} \alpha_e \cos \theta. \quad (47)$$

The higher harmonic is given by

$$j_{s(2\omega)}^z = -e \frac{\tau}{\hbar^2} \frac{q\sigma^0}{\omega} \frac{|E|^2(1 - \zeta^2)}{(1 + \zeta^2)^2} \alpha_e \cos \theta. \quad (48)$$

#### A. Parameters used for RuO<sub>2</sub>

In the main text, we consider RuO<sub>2</sub> as the metallic altermagnet. Ref. [10] has measured the room temperature conductivity of RuO<sub>2</sub> thin films to be  $\sigma_e \approx 10^6$  S/m. Additionally, they measure a Hall conductivity of  $0.5 \mu\Omega\text{cm}$  at  $\mu H = 12$  T, which gives an electron density of  $n_e = 1.5 \times 10^{28} \text{ m}^{-3}$ .

The electron dispersion we approximate with  $m_e \approx 0.4m_0$ , and the spin splitting with  $\alpha_e \approx 0.4\hbar^2/m_e$ . Additionally, the estimate of  $R$  [Eq. (46)] requires the spin-independent density of states at the Fermi level, which can be found from *ab initio* calculations to be  $D_{\alpha=0}(\epsilon_F) \approx 13 \text{ eV}^{-1} \text{ nm}^{-3}$ .

<sup>3</sup> Note that we have multiplied with the electron charge to obtain a current density, i.e., it has units A/m<sup>2</sup>.

### III. Second order magnon response to a surface acoustic wave

We now consider the response of the magnetic excitations, the magnons, of the antiferromagnetic ordering of an altermagnet. A single magnon wavepacket with frequency  $\omega_{\mathbf{k}}$  and wave vector  $\mathbf{k}$  can experience a force by a SAW with frequency  $\omega$  and wave vector  $\mathbf{q}$ —as long as the variation of the SAW is on time and length scales much longer and slower than the wavepacket's, i.e., if  $\omega < \omega_{\mathbf{k}}$  and  $\mathbf{q} < \mathbf{k}$ . Conversely, if the variation of the SAW is on time and length scales much shorter and faster than the wavepacket's the SAW can scatter the magnon wavepacket into a new state with wavevector  $\mathbf{k} + \mathbf{q}$  and frequency  $\omega_{\mathbf{k}} + \omega$ . In the intermediate regime, where the time and length scales of the wavepacket and SAW are comparable, both processes can occur.

There are three possible scattering mechanisms: hybridization, Cherenkov scattering and confluence processes [11]. Importantly, hybridization requires that  $\omega_{\mathbf{q}} = \omega_{m;\mathbf{k}}$  and  $\mathbf{q} = \mathbf{k}$ , Cherenkov scattering requires  $\omega_{\mathbf{q}} = \omega_{m;\mathbf{k}+\mathbf{q}} - \omega_{m;\mathbf{k}}$ , and confluence requires  $\omega_{\mathbf{q}} = \omega_{m;\pm\mathbf{k}} - \omega_{m;\mathbf{q}\mp\mathbf{k}}$ . However, given the linear dispersion of antiferromagnetic magnons for long wavelengths in combination with the linear dispersion of the SAW, none of these requirements can be met, and thus the direct scattering processes are not allowed. The main interaction of the SAW with the magnons is therefore through a force  $\mathbf{F}$ , which acts on the short wavelength magnons. We therefore continue by including only the force  $\mathbf{F}$  in the Boltzmann equation.

In addition, we will parameterize the non-equilibrium magnon response by the magnon chemical potential  $\mu_m$ , which is well-justified on time scales set by the exchange-driven magnon-magnon interaction. Additionally, the antiferromagnetic ordering of the magnetic moments allows for the angular momentum-conserving interband scattering of magnons. However, it has been previously shown that these processes are relatively minor, and do not contribute to the magnon spin conductivity [12]. We therefore neglect them here, but we expect that the reintroduction of these terms would not affect the main results of this work—since these scattering processes conserve angular momentum.

We now obtain the Boltzmann equation for the magnon distribution function  $f_m^\sigma$  as [note that this Boltzmann equation is only valid for  $k \gg q$ ]

$$\partial_t f_m^\sigma + v_{m;\mathbf{k}}^\sigma \cdot \nabla_{\mathbf{r}} f_m^\sigma + \hbar^{-1} \mathbf{F}(\mathbf{r}, t, \mathbf{k}) \cdot \nabla_{\mathbf{k}} f_m^\sigma = -\frac{f_m^\sigma - \langle f_m^\sigma \rangle}{\tau_{\mathbf{k}}} \quad (49)$$

In what follows, much of the derivation will follow the same lines as in Section I. Additionally, we will suppress the  $m$  label in the subscript for notational clarity where possible. We can then directly write down

$$f_1^\sigma = \frac{-\zeta_k \tau_{\mathbf{k}} \partial_{\epsilon_{\mathbf{k}}} f_0^\sigma \mathbf{F}_{\mathbf{k}} \cdot \mathbf{v}_{\mathbf{k}}^\sigma / \hbar + n_1^\sigma \frac{\partial f_0}{\partial n}}{1 - i\alpha_{\mathbf{k}}}, \quad (50)$$

where  $\alpha_{\mathbf{k}} \equiv \tau_{\mathbf{k}}(\omega + \mathbf{v}_{\mathbf{k}} \cdot \mathbf{q})$  and have allowed the relaxation time  $\tau_{\mathbf{k}}$  to be wave vector dependent. We follow the same analysis as before, arriving at

$$n_1^\sigma = \zeta_k \sum_{\alpha\beta} \frac{q^\alpha \sigma_{m;\alpha\beta}^\sigma F_{\mathbf{k}}^\beta}{\omega - q_\alpha R_{\alpha}^\sigma}, \quad (51)$$

where we note that there is no analogue of the self-induced electric field for the magnons. The conductivity tensor for magnons is defined as

$$\sigma_{m;\alpha\beta}^\sigma \equiv - \int \frac{d\mathbf{k}}{(2\pi)^d} \frac{\tau_{\mathbf{k}} v_{\mathbf{k}\alpha}^\sigma v_{\mathbf{k}\beta}^\sigma}{1 - i\alpha_{\mathbf{k}\sigma}} \frac{\partial f_0^\sigma}{\partial \epsilon_{\mathbf{k}\sigma}}, \quad (52)$$

and the magnon diffusion vector is

$$R_{m;\alpha}^\sigma \equiv -\frac{\partial \mu}{\partial n} \int \frac{d\mathbf{k}}{(2\pi)^d} \frac{v_{\mathbf{k}\alpha}^\sigma}{1 - i\alpha_{\mathbf{k}\sigma}} \frac{\partial f_0^\sigma}{\partial \epsilon_{\mathbf{k}\sigma}}. \quad (53)$$

The second order response follows then as [analogous to Eq. (26)]

$$j_{(0)\alpha}^\sigma = \frac{1}{2} \sum_{\beta} \text{Re} \int \frac{d\mathbf{k}}{(2\pi)^d} \tau_{\mathbf{k}} \left( F_{\mathbf{k}}^\beta \frac{\partial v_{\mathbf{k}\alpha}^\sigma}{\partial k_\beta} f_1^\sigma + v_{\mathbf{k}\alpha}^\sigma \frac{\partial F_{\mathbf{k}}^\beta}{\partial k_\beta} f_1^\sigma \right), \quad (54)$$

where the second term comes from the fact that the force is now  $\mathbf{k}$  dependent. The diffusion current reads as

$$j_{(0)\alpha}^\sigma = -\frac{\partial \mu}{\partial n} \frac{1}{2\hbar} \frac{q \sigma_0^{\sigma m}}{\omega} \int \frac{d\mathbf{k}}{(2\pi)^d} \tau_{\mathbf{k}} \left( \frac{\partial v_{\mathbf{k}\alpha}^\sigma}{\partial k_\beta} |F_{\mathbf{k}}^\beta|^2 + v_{\mathbf{k}\alpha}^\sigma F_{\mathbf{k}}^\beta \frac{\partial F_{\mathbf{k}}^\beta}{\partial k_\beta} \right) \frac{\partial f_0}{\partial \epsilon_{\mathbf{k}}}. \quad (55)$$

In what follows, we will approximate the relaxation time as  $\mathbf{k}$ -independent, i.e.,  $\tau_{\mathbf{k}} \approx \tau$  [13].

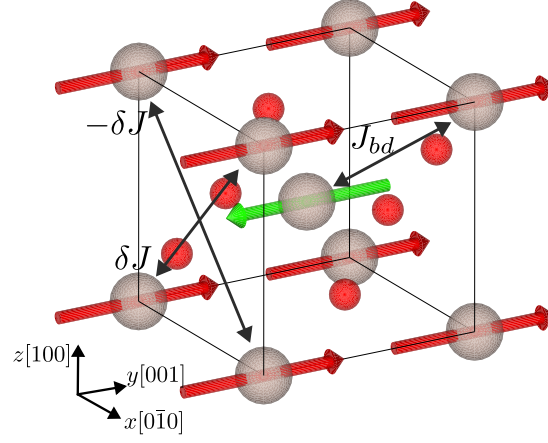

FIG. 1. Crystal structure of a rutile-based insulating altermagnet. The antiferromagnetic ordering of the magnetic cations (grey) is indicated by the arrows. Nearest-neighbor magnetic atoms are coupled by  $J_{bd}$ . Because the non-magnetic anions (red) break the crystal symmetry, the second neighbor magnetic atoms are coupled by an altermagnetic coupling  $\delta J$ , which has opposite values on the diagonals. The crystallographic directions are indicated, as well as the lattice constant  $a$ . Note that for simplicity we have assumed a cubic unit cell, whereas most rutiles are orthorhombic.

#### IV. Insulating altermagnet

The strain induced by the SAW modulates the exchange interaction  $J_{ij}$  between spins  $i$  and  $j$ , by modulating the bond length. Since coupling of the SAW to the magnons depends on the specific crystal structure, we specify here first the insulating altermagnetic model we consider. Inspired by  $\text{RuO}_2$  we take a rutile-based crystal structure, and we include only the minimal couplings to capture the  $d$ -wave altermagnetic symmetries, as shown in Fig. 1. Additionally, we will assume for simplicity that the unit cell is cubic, with lattice constant  $a$ .

The spin Hamiltonian for the spins  $\mathbf{S}_i$  on site  $i$  is given by

$$\mathcal{H} = \sum_{ij} J_{ij} \mathbf{S}_i \cdot \mathbf{S}_j, \quad (56)$$

where  $J_{ij}$  is the exchange interaction strength between sites  $i$  and  $j$ . Similar to the electronic case, the crystal environment generates exchange interactions which are unequal along the face diagonals [14].

We now perform the Holstein-Primakoff transformation, assuming a collinear anti-aligned ordering,

$$S_{i,A}^- \sim \sqrt{2S} a_i; \quad S_{i,A}^z = S - a_i^\dagger a_i; \quad S_{i,B}^- \sim \sqrt{2S} b_i^\dagger; \quad S_{i,B}^z = -S + b_i^\dagger b_i \quad (57)$$

to obtain the linear spin-wave Hamiltonian

$$H^{(2)} = \sum_{ij} A_{ij} a_i^\dagger a_j + A_{ij} b_i^\dagger b_j + B_{ij} (b_i a_j + b_i^\dagger a_j^\dagger), \quad (58)$$

where

$$A_{ij} = S \left( \delta_{ij} \sum_n J_{in} - J_{ij} \right) \quad (59)$$

$$B_{ij} = -S J_{ij}^{bd} \quad (60)$$

We now apply a rotation to the frame within which the SAW is propagating along the  $x$  direction. Specifically, we perform the rotation  $\mathbf{r}' = \mathcal{R} \mathbf{r}$ , with

$$\mathcal{R} = \begin{pmatrix} \cos \theta & -\sin \theta & 0 \\ \sin \theta & \cos \theta & 0 \\ 0 & 0 & 1 \end{pmatrix}. \quad (61)$$



After applying a Fourier transformation  $b_i = \frac{1}{\sqrt{N}} \sum_{\mathbf{k}} e^{i\mathbf{r}'_i \cdot \mathbf{k}} b_{\mathbf{k}}$ ,  $a_i = \frac{1}{\sqrt{N}} \sum_{\mathbf{k}} e^{i\mathbf{r}'_i \cdot \mathbf{k}} a_{\mathbf{k}}$ , we obtain

$$H^{(2)} = \sum_{\mathbf{k}} \psi_{\mathbf{k}}^\dagger \begin{pmatrix} A + \delta A_{\mathbf{k}} & 0 & 0 & B_{\mathbf{k}} \\ 0 & A - \delta A_{\mathbf{k}} & B_{\mathbf{k}} & 0 \\ 0 & B_{\mathbf{k}} & A + \delta A_{\mathbf{k}} & 0 \\ B_{\mathbf{k}} & 0 & 0 & A - \delta A_{\mathbf{k}} \end{pmatrix} \psi_{\mathbf{k}}; \quad \psi_{\mathbf{k}} \equiv \begin{pmatrix} a_{\mathbf{k}} \\ b_{\mathbf{k}} \\ a_{-\mathbf{k}}^\dagger \\ b_{-\mathbf{k}}^\dagger \end{pmatrix} \quad (62)$$

where

$$A_{\mathbf{k}} = 8S J_{bd} \quad (63)$$

$$\delta A_{\mathbf{k}} = 4S \delta J a^2 k_z (k_x \cos \theta - k_y \sin \theta) \quad (64)$$

$$B_{\mathbf{k}} = S J_{bd} (8 - (ka)^2), \quad (65)$$

and we have expanded up to first order in  $k_\eta a$ , where  $\eta \in \{x, y, z\}$ .

To find the long-wavelength magnon dispersion, we apply a Bogoliubov transformation

$$a_{\mathbf{k}} = \cosh \phi \alpha_{\mathbf{k}} + \sinh \phi \beta_{-\mathbf{k}}^\dagger \quad (66)$$

$$b_{-\mathbf{k}}^\dagger = \sinh \phi \alpha_{\mathbf{k}} + \cosh \phi \beta_{-\mathbf{k}}^\dagger \quad (67)$$

where we have dropped the corrections to the ground state energy and defined

$$\tanh 2\phi \equiv -\frac{B_{\mathbf{k}}}{A}. \quad (68)$$

The Hamiltonian then becomes diagonal,

$$H^{(2)} = \hbar \sum_{\mathbf{k}} \omega_{\mathbf{k}}^+ \alpha_{\mathbf{k}}^\dagger \alpha_{\mathbf{k}} + \omega_{\mathbf{k}}^- \beta_{\mathbf{k}}^\dagger \beta_{\mathbf{k}} \quad (69)$$

where

$$\hbar \omega_{\mathbf{k}}^\pm = \sqrt{A^2 - B_{\mathbf{k}}^2} \pm \delta A_{\mathbf{k}} = v_s k + \sigma \alpha_m k_z (k_x \cos \theta - k_y \sin \theta) \quad (70)$$

is the magnon dispersion relation, where  $\sigma$  labels the positive and negative chirality magnon modes—which refer to as the magnon spin for simplicity. Here,  $v_s \equiv 4J_{bd} S a$  is the isotropic magnon spin velocity and  $\alpha_m \equiv 4S a^2 \delta J$ .

We can now evaluate

$$\hbar \mathbf{v}_{\mathbf{k}}^\sigma = v_s \hat{\mathbf{k}} + \sigma \alpha_m [k_z \cos \theta \hat{\mathbf{x}} - k_z \sin \theta \hat{\mathbf{y}} + (k_x \cos \theta - k_y \sin \theta) \hat{\mathbf{z}}] \quad (71)$$

and thus

$$\frac{\hat{\mathbf{z}} \cdot \partial(\mathbf{v}_{\mathbf{k}z}^\uparrow - \mathbf{v}_{\mathbf{k}z}^\downarrow)}{\partial k_x} = 2\hbar^{-1} \alpha_m \cos \theta. \quad (72)$$

Following this rotation—as in the electron case—we also require the magnon spin conductivity  $\sigma_{xx}^{\alpha=0}$ . To evaluate this, we replace the Bose-Einstein function with the Maxwell-Boltzmann distribution find

$$\sigma_0 = -\tau \int \frac{d\mathbf{k}}{(2\pi)^d} (v_x)^2 \left. \frac{\partial f_0^\sigma}{\partial \epsilon_{\mathbf{k}\sigma}} \right|_{\alpha_m=0} = \frac{\tau (k_B T)^2}{3\hbar^2 \pi^2 v_s}. \quad (73)$$

We note however that because magnons are bosonic particles, all magnons could contribute to transport—in stark contrast to electronic systems, where only the electrons around the Fermi level contribute. Additionally, it is notoriously difficult to accurately measure the magnon relaxation time  $\tau$ , which could vary strongly as a function of magnon wave number, and therefore Eq. (73) is of limited practical value. In the main text we therefore assume a magnon conductivity measured experimentally in antiferromagnetic thin films.<sup>4</sup>

<sup>4</sup> Note that the fact that  $\tau$  is potentially a complicated function of  $\mathbf{k}$  also implies that measuring  $\sigma_0$  experimentally does not allow on to calculate  $\tau$ . In practice this means that both  $\tau$  and  $\sigma_0$  will be phenomenological fitting parameters, although their order of magnitude can of course be estimated, which is what we use in the main text.

Additionally, we determine

$$\frac{\partial \mu}{\partial n} = - \left[ \int \frac{d\mathbf{k}}{(2\pi)^3} \frac{\partial f}{\partial \epsilon_{\mathbf{k}}} \right]^{-1} = \left[ \frac{1}{k_B T} \int \frac{d\mathbf{k}}{(2\pi)^3} e^{-v_s k / k_B T} \right]^{-1} = \frac{\pi^2 v_s^3}{(k_B T)^2} \quad (74)$$

where we neglect again the altermagnetic splitting, following the same arguments as above. Finally, the diffusion vector along  $q$  is given by

$$R = -iq \frac{\partial \mu}{\partial n} \sigma_0. \quad (75)$$

#### A. Parameters used in the main text

In the main text, we take the exchange parameters from *ab initio* calculations for RuO<sub>2</sub> [14]:  $J_{bd}S = 2.5$  meV and  $\delta JS = 1.5$  meV. This gives  $v_s = 45$  meV Å and  $\alpha_m = 1.2$  meV nm<sup>2</sup>.

#### V. Magnon strain coupling

We first derive the effective force on the magnons due to strain modulating the exchange coupling. We start from the exchange Hamiltonian

$$\mathcal{H}_J = \sum_{ij} J_{ij}(r_{ij}) \mathbf{S}_i \cdot \mathbf{S}_j, \quad (76)$$

and assume that the exchange strength depends on the bond length, such that we can expand the exchange interaction as

$$J_{ij} = J + \frac{\partial J}{\partial r_{ij}} \cdot \mathbf{r}_{ij}. \quad (77)$$

Specificially, we assume that the exchange interaction changes only as a function of distance  $r_{ij} \equiv |\mathbf{r}_{ij}|$ , such that we can approximate

$$r_{ij}^\alpha \approx \sum_{\beta} a_{ij} \tau_{ij}^\alpha \partial_\alpha u_i^\beta, \quad (78)$$

where  $\boldsymbol{\tau}$  is the unit vector connecting the two sites and  $a$  is the bond length. Therefore, we obtain

$$J_{ij} \approx J_{ij}^0 + J'_{ij} a_{ij} \sum_{\alpha\beta} \tau_{ij}^{\alpha\beta} u_i^{\alpha\beta}, \quad (79)$$

where  $u_i^{\alpha\beta} \equiv \partial_\alpha u_i^\beta$  are the components of the stress tensor,  $J_{ij}^0 \equiv J_{ij}(a_{ij})$  and  $J'_{ij} \equiv \partial_r J|_{r=a_{ij}}$ . Furthermore, we have defined the tensor  $\tau_{ij}^{\alpha\beta} = \tau_{ij}^\alpha \tau_{ij}^\beta$ . We now use the magnetic Grüneisen parameter [15],

$$\beta_{ij} \equiv \frac{J'_{ij} a}{3J_{ij}}, \quad (80)$$

to write

$$J_{ij} \approx J_{ij}^0 + 3J_{ij}^0 \beta_{ij} \sum_{\alpha\beta} \tau_{ij}^{\alpha\beta} u_{\alpha\beta}^i. \quad (81)$$

Finally, we note that typically  $\beta \approx -10/3$ , for a wide range of magnetic materials [16].

Following the derivation above, we can now write an effective Hamiltonian, where the strain tensor  $u_i^{\alpha\beta}$  is coupled to the exchange energy. In addition, as was also discussed in Section III, the SAW wave vector  $\mathbf{q}$  is much smaller than the magnon wavevectors  $\mathbf{k}$  which participate in transport, the SAW frequency is much smaller than the thermal magnon frequencies. We can then treat the SAW quasiclassically, i.e., as quasistatic and quasiuniform. We thus write the strain coupling as an effective Hamiltonian,

$$H^{\text{strain}} = \sum_{ij} A_{ij}^{\text{strain}} a_i^\dagger a_i + A_{ij}^{\text{strain}} b_i^\dagger b_i + B_{ij}^{\text{strain}} (b_i a_i + b_i^\dagger a_i^\dagger), \quad (82)$$

where

$$A_{ij}^{\text{strain}} = 3S \sum_{\alpha\beta} \left( \delta_{ij} \sum_n J_{in} \beta_{in} \tau_{in}^{\alpha\beta} u_i^{\alpha\beta} - J_{ij} \beta_{ij} \tau_{ij}^{\alpha\beta} u_i^{\alpha\beta} \right) \quad (83)$$

$$B_{ij}^{\text{strain}} = -3S J_{ij}^{bd} \beta_{ij} \tau_{ij}^{\alpha\beta} u_i^{\alpha\beta}. \quad (84)$$

Continuing in the quasistatic approximation, we assume the stress tensor  $u_i^{\alpha\beta}$  to be slowly varying on the time and length scale of the magnons, and thus we can now perform a Fourier transformation for the magnon operators  $a_i, b_i$ , but not for the stress tensor. A Bleustein-Gulyaev surface acoustic wave has only two non-zero components of the stress tensor,  $u_{xy}$  and  $u_{yz}$ , such that we obtain

$$H_{(2)}^{\text{strain}}(\mathbf{r}, t) = \sum_{\mathbf{k}} \psi_{\mathbf{k}}^{\dagger} \begin{pmatrix} 0 & 0 & 0 & B_{\mathbf{k}}^{\text{strain}} \\ 0 & 0 & B_{\mathbf{k}}^{\text{strain}} & 0 \\ 0 & B_{\mathbf{k}}^{\text{strain}} & 0 & 0 \\ B_{\mathbf{k}}^{\text{strain}} & 0 & 0 & 0 \end{pmatrix} \psi_{\mathbf{k}}; \quad (85)$$

where

$$B_{\mathbf{k}}^{\text{strain}} = -3u_{xy}(\mathbf{r}, t) S a^2 \beta_{bd} J_{bd} \cos 2\theta \left[ 2k_x k_y \cos 2\theta + (k_x^2 - k_y^2) \sin 2\theta \right] - 6u_{yz}(\mathbf{r}, t) S a^2 \beta_{bd} J_{bd} k_y k_z \quad (86)$$

and  $\beta_{\eta}$  is the Grüneisen parameter belonging to the exchange along bond  $\eta \in [bd, d]$ . We neglected the contributions from  $\delta J \beta_d$ , because  $\delta J < J_{bd}$ .<sup>5</sup> Note that the four-fold symmetry in  $B_{\mathbf{k}}^{\text{strain}}$  is due to the crystal symmetry, and is not related to the alternating band splitting.

We apply the Bogoliubov transformation, Eqs. (66,67), such that the strain Hamiltonian is given by<sup>6</sup>

$$H_{(2)}^{\text{strain}}(\mathbf{r}, t) = \sum_{\mathbf{k}} \epsilon_{\mathbf{k}}^{\text{strain}} \left( \alpha_{\mathbf{k}}^{\dagger} \alpha_{\mathbf{k}} + \beta_{\mathbf{k}}^{\dagger} \beta_{\mathbf{k}} \right), \quad (87)$$

where

$$\epsilon_{\mathbf{k}}^{\text{strain}} = 6u_{xy}(\mathbf{r}, t) \beta_{bd} v_s \cos 2\theta \frac{2k_x k_y \cos 2\theta + (k_x^2 - k_y^2) \sin 2\theta}{k} + 12u_{yz}(\mathbf{r}, t) v_s \frac{k_y k_z}{k}. \quad (88)$$

The force on a Bogoliubov quasiparticle, i.e., on a magnon, with wavelength  $\mathbf{k}$  is now given by

$$\mathbf{F}(\mathbf{r}, t) = -\nabla_{\mathbf{r}} H_{(2)}^{\text{strain}}(\mathbf{r}, t). \quad (89)$$

Within this rotated frame, the SAW propagates along the  $\hat{x}$  direction, such that  $u_y = u_0 e^{-|z|/\lambda_q} e^{iqx - i\omega t}$  and thus

$$u_{xy} = iqu_0 e^{iqx - i\omega t}; \quad u_{yz} = -u_0 \lambda_q^{-1} e^{iqx - i\omega t}. \quad (90)$$

Here  $u_0$  is the atomic displacement of the SAW,  $\lambda_q$  is the deformation decay length and we have neglected the decay of the deformation, since  $\lambda_q \gg d$  with  $d$  the thickness of the film, and thus  $e^{-|z|/\lambda_q} \approx 1$ . Finally, we make use of the fact that  $\lambda_q^{-1} = \varrho q$  to write

$$u_{xy} = iqu_0 e^{iqx - i\omega t}; \quad u_{yz} = -u_0 \varrho e^{iqx - i\omega t}, \quad (91)$$

where  $\varrho$  is a dimensionless piezoelectric coupling factor. We refer the reader to Section VII for more details.

From Eq. (89) we now obtain the forces along the propagation direction of the SAW as

$$F_x = iqu_0 \epsilon_{\mathbf{k}}^{\text{strain}}, \quad (92)$$

where  $\theta$  is the angle of the SAW with the crystallographic axis. Importantly, the forces are dependent on the magnon wave vector, i.e. on  $\mathbf{k}$ —in contrast to the electric field for the electrons, which is constant in  $\mathbf{k}$ -space. Note that we neglect here the forces along the  $z$ -axis, as discussed in more detail in Section VIII.

<sup>5</sup> Additionally, the coupling to strain is expected to be proportional to the bond length, and thus  $\beta_d < \beta_{bd}$ .

<sup>6</sup> Note that the resulting strain also happens to be diagonal after Bogoliubov transformation, but this is not necessarily guaranteed.

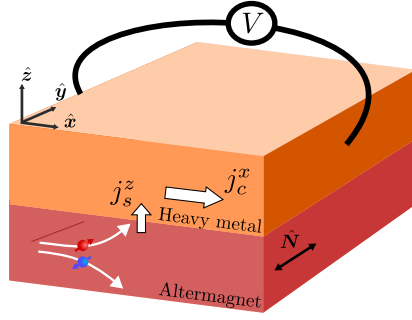

FIG. 2. The detection of the transverse spin current using the inverse spin Hall effect in the heavy metal. The spin current  $j_s^z$  along  $z$  is polarized along the Néel vector. This will be converted to a charge current along  $x$  through the inverse spin Hall effect, which can be detected as a voltage along  $x$ .

We are now in the position to evaluate Eq. (55). As a reminder, we assume that the relaxation time  $\tau_k$  is  $k$ -independent, such that what remains is to evaluate the integral

$$\int \frac{d\mathbf{k}}{(2\pi)^d} \left( \frac{(\mathbf{v}_\mathbf{k}^\uparrow - \mathbf{v}_\mathbf{k}^\downarrow) \cdot \hat{\mathbf{z}}}{\partial k_x} |F_x|^2 + (\mathbf{v}_\mathbf{k}^\uparrow - \mathbf{v}_\mathbf{k}^\downarrow) \cdot \hat{\mathbf{z}} \frac{\partial F_x}{\partial k_x} F_x^* \right) \frac{\partial f_0}{\partial \epsilon_\mathbf{k}} \quad (93)$$

from Eq. (55). The second part of the integral [containing  $\mathbf{v}_\mathbf{k}^\sigma \cdot \hat{\mathbf{z}} \frac{\partial F_x}{\partial k_x} F_x^*$ ] vanishes, because  $\mathbf{v}_\mathbf{k}^\sigma \cdot \hat{\mathbf{z}}$  is odd in  $k_z$ , whilst  $\partial k_x F_x$  is even in  $k_z$ . The remaining integral can be performed and we find that

$$\int \frac{d\mathbf{k}}{(2\pi)^d} \left( \frac{(\mathbf{v}_\mathbf{k}^\uparrow - \mathbf{v}_\mathbf{k}^\downarrow) \cdot \hat{\mathbf{z}}}{\partial k_x} |F_x|^2 \right) \frac{\partial f_0}{\partial \epsilon_\mathbf{k}} = 2q^4 u_0^2 \frac{\sigma \alpha_m \beta_{bd}^2 (k_B T)^4}{\hbar (\pi v_s)^3} h(\theta) \cos \theta, \quad (94)$$

where  $h(\theta) = 30.7 + 0.834\varrho + 38.6 \cos 4\theta + 8.11 \cos 8\theta$  is a function with rational prefactors, which follow from the integration over the space  $\mathbf{k}$ .<sup>7</sup> For simplicity, we give their rounded values. Note that the four and eight fold rotational symmetry is the result of the second-order nature of the response, in combination with the four-fold in-plane rotational symmetry of the  $J_{bd}$  bonds. Finally, the piezoelectric coupling factor  $\varrho$  appears in  $h(\theta)$  because it relates the two amplitudes of the two strain components  $u_{xy}$  and  $u_{yz}$  to each other [see Eq. (91)].

We now obtain the transverse spin current,

$$j_z^{s(0)} = -\frac{\partial \mu}{\partial n} \frac{\tau}{\hbar^2} \frac{\sigma_0 q}{\omega} \frac{F_{\text{eff}}^2}{1 + \chi_m} \alpha_m h(\theta) \cos \theta, \quad (95)$$

where we have defined

$$F_{\text{eff}} \equiv q^2 u_0 \frac{\beta_{bd} (k_B T)^2}{(\pi v_s)^{3/2}} \quad (96)$$

and  $\chi_m \equiv q^2 \sigma_m^0 (\partial \mu_m / \partial n_m) / \omega$ , which measures the screening of the induced magnon current through diffusion. Note that for the parameters used in the main text we have that  $\chi_m \approx 10^{-4}$  for  $\omega/2\pi = 0.5$  GHz. Additionally, we obtain a second order harmonic as

$$j_z^{s(2\omega)} = -\frac{\partial \mu}{\partial n} \frac{\tau}{\hbar^2} \frac{\sigma_0 q}{\omega} \frac{F_{\text{eff}}^2}{1 + \chi_m} \alpha_m h(\theta) \cos \theta. \quad (97)$$

## VI. Detecting the transverse spin current with a heavy metal

In the geometry as suggested in this work, there is a spin current flowing along the  $z$ -axis, with a polarization along the Néel vector, which we assume to lie along the  $y$ -axis. To detect this spin current we propose to use the inverse spin Hall effect in an

<sup>7</sup> The contributions from the two strain components separate, because in the strain Hamiltonian  $u_{yz}$  only appears with terms odd in  $k_z$ , whereas  $u_{xy}$  appears only with terms even in  $k_z$ , such that their product vanishes once integrated.

adjacent heavy metal, as shown in Fig. 2. Specifically, placing a heavy metal on top of the altermagnetic thin film will allow the spin current to enter into the heavy metal, where it will be converted in a charge current which can be detected by attaching leads to the normal metal.

The spin current  $j_s$  along  $z$  will be converted in a charge current  $j_c$  along  $x$  through the inverse spin Hall effect as

$$\mathbf{j}_c = \theta_S j_s \hat{\mathbf{x}}. \quad (98)$$

This charge current will be then converted into a voltage  $V_{HM}$  if leads are attached as

$$V_{HM} = j_c A R, \quad (99)$$

where  $A = l_x \times l_y$  is the area of the heavy metal with sides  $l_x, l_y$  and  $R = \rho l_x / (l_y d)$ , with  $\rho$  the resistivity of the heavy metal.

## VII. Details of a Bleustein-Gulyaev surface acoustic wave

A Bleustein-Gulyaev (BG) surface acoustic wave (SAW) [2, 3] travelling along the  $x$ -axis is described by

$$u_y = u_0 e^{-|z|/\lambda_q} e^{i(qx - \omega t)} \quad (100)$$

$$\phi = \phi_0 e^{-|z|/\lambda_q} e^{i(qx - \omega t)}, \quad (101)$$

where  $u_y$  is the displacement along the  $y$ -axis and  $\phi$  is the electric potential. This gives the strain components

$$u_{xy} = i u_0 q e^{-|z|/\lambda_q} e^{i(qx - \omega t)} \quad (102)$$

$$u_{xz} = -u_0 / \lambda_q e^{-|z|/\lambda_q} e^{i(qx - \omega t)}. \quad (103)$$

Here,  $\lambda_q^{-1} = \varrho q$  is the deformation decay length with  $\varrho^{-1} = \epsilon \epsilon_0 \bar{c}_{44} / e_{15}^2$ ,  $\epsilon_{PZ}$  is the dielectric constant of the piezoelectric,  $e_{15}$  is the piezoelectric constant and  $\bar{c}_{44} \equiv c_{44} + e_{15}^2 / \epsilon_{PZ}$  is the piezoelectrically stiffened elastic constant, with  $c_{44}$  the elastic constant.

Finally, the deformation amplitude and potential are related as  $\phi_0 = c_{PZ} u_0$ , with

$$c_{PZ} = \frac{e_{15}}{\epsilon_0 \epsilon_{PZ}} \quad (104)$$

and the dispersion relation is given as

$$s^2 = \frac{\bar{c}_{44}}{\rho} (1 - \varrho^2) \quad (105)$$

such that  $\omega = sq$ . Finally, the SAW intensity is given by

$$I_0 = s \rho \int_{-\infty}^0 dz |\dot{u}_y(x, z)|^2 \quad (106)$$

$$= \omega s^2 u_0^2 \rho \frac{\epsilon \epsilon_0}{2 e_{15}^2}. \quad (107)$$

We assume the BG SAW to travel in the piezoelectric LiNbO<sub>3</sub> (lithium niobate), for example along the  $X$  axis of a 60° rotated  $Y$ -cut crystal [17]. For LiNbO<sub>3</sub> we have dielectric constant  $\epsilon_{11} = 44$ ; the piezoelectric constant is  $e_{15} = \epsilon_0 \epsilon_{11} / d_{15}$ , where  $d_{15} = 7.0 \times 10^{-11}$  C/N, such that  $e_{15} = 6$  C/m<sup>2</sup>, the elastic constant is  $c_{44} = 6 \times 10^{10}$  N/m<sup>2</sup> and the mass density is  $\rho = 5 \times 10^3$  kg/m<sup>3</sup> [18]. For these values, we have that  $s \approx 4$  km/s. Additionally, we can calculate the average deformation across a unit cell as  $u_y|_x - u_y|_{x+a} \approx q u_0 a \approx 10^{-6} a$ .

## VIII. Effect of the electric field and deformation force along the $z$ -axis

In this work, we have neglected the effect of the BG SAW piezoelectric field along  $z$  on the electronic spin current along  $z$ . In this section we qualitatively discuss the effects of reintroducing these out of plane components on the acoustic spin splitter, and show that can rightfully be ignored.

Importantly, we consider here an altermagnetic spin-split plane oriented along the  $xz$  plane. Therefore, a force along  $z$  will only drive a spin current along  $x$  and thus not contribute to the out-of-plane spin current. The force along  $z$  will also drive a charge current along  $z$ , which could enter the heavy metal—but since the voltage is only measured along  $x$  this will not be detected.

For the magnons, we have neglected the force along the  $z$ -axis, defined through Eq. (89). The qualitative effect of this force is similar to the electric field along  $z$  for the electrons, and the above considerations therefore also apply.

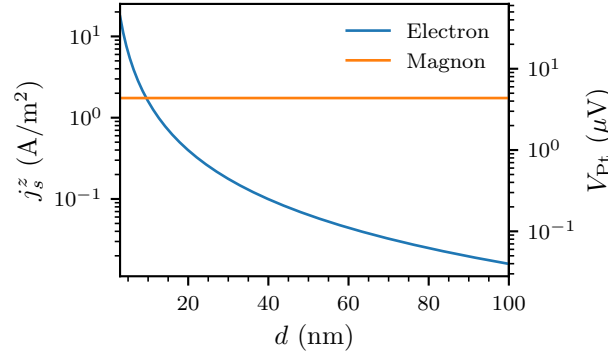

FIG. 3. The transverse spin current carried by electrons and magnons, as a function of the thin film thickness  $d$ . Increasing the thickness screens the piezoelectric field and thus suppresses the electron spin current. The deformation is not screened, and thus the magnon response is independent of thickness.

### IX. Thickness dependency

In Fig. 3 we show how the thickness of the thin film affects the generated spin current. We observe that the electron spin current magnitude decreases for thicker films, whereas the magnon spin current stays constant. This is directly related to the electron screening  $\zeta_e$ , which is proportional to the velocity of charge spreading,  $v^*$ , which is in turn proportional to the thickness, and thus  $1/(1 + \zeta^2) \propto d^{-2}$ , which is exactly in scaling we observe in Fig. 3. The magnon diffusive screening, parameterized by  $\chi_m$ , is independent of thickness and thus does not play a role here.

- 
- [1] M. P. Marder, *Condensed matter physics*, 2nd ed. (Wiley, Hoboken, N.J, 2010).
  - [2] J. L. Bleustein, A new surface wave in piezoelectric materials, *Applied Physics Letters* **13**, 412 (1968).
  - [3] Yu. V. Gulyaev, Electroacoustic surface waves in solids, *JETP Letters* **9**, 37 (1969).
  - [4] K. Sonowal, A. V. Kalameitsev, V. M. Kovalev, and I. G. Savenko, Acoustoelectric effect in two-dimensional Dirac materials exposed to Rayleigh surface acoustic waves, *Physical Review B* **102**, 235405 (2020).
  - [5] A. V. Kalameitsev, V. M. Kovalev, and I. G. Savenko, Valley Acoustoelectric Effect, *Physical Review Letters* **122**, 256801 (2019).
  - [6] T. Ando, A. B. Fowler, and F. Stern, Electronic properties of two-dimensional systems, *Reviews of Modern Physics* **54**, 437 (1982).
  - [7] J. Lee and H. N. Spector, Dielectric function for a quasi-two-dimensional semiconducting system, *Journal of Applied Physics* **54**, 6989 (1983).
  - [8] C. Kittel and C. Y. Fong, *Quantum theory of solids*, 2nd ed. (Wiley, New York, 1987).
  - [9] N. W. Ashcroft and N. D. Mermin, *Solid State Physics* (Saunders College Publishing, 1976).
  - [10] T. Tschirner, P. Keßler, R. D. Gonzalez Betancourt, T. Kotte, D. Krieger, B. Büchner, J. Dufouleur, M. Kamp, V. Jovic, L. Smejkal, J. Sinova, R. Claessen, T. Jungwirth, S. Moser, H. Reichlova, and L. Veyrat, Saturation of the anomalous Hall effect at high magnetic fields in altermagnetic RuO<sub>2</sub>, *APL Materials* **11**, 101103 (2023).
  - [11] A. Rückriegel, S. Streib, G. E. W. Bauer, and R. A. Duine, Angular Momentum Conservation and Phonon Spin in Magnetic Insulators, *Physical Review B* **101**, 104402 (2020).
  - [12] R. E. Troncoso, S. A. Bender, A. Brataas, and R. A. Duine, Spin transport in thick insulating antiferromagnetic films, *Physical Review B* **101**, 054404 (2020).
  - [13] S. M. Rezende, R. L. Rodríguez-Suárez, and A. Azevedo, Diffusive magnonic spin transport in antiferromagnetic insulators, *Physical Review B* **93**, 054412 (2016).
  - [14] L. Šmejkal, A. Marmodoro, K.-H. Ahn, R. González-Hernández, I. Turek, S. Mankovsky, H. Ebert, S. W. D'Souza, O. Šipr, J. Sinova, and T. Jungwirth, Chiral Magnons in Altermagnetic RuO<sub>2</sub>, *Physical Review Letters* **131**, 256703 (2023).
  - [15] D. Bloch, The 10/3 law for the volume dependence of superexchange, *Journal of Physics and Chemistry of Solids* **27**, 881 (1966).
  - [16] S. Streib, N. Vidal-Silva, K. Shen, and G. E. W. Bauer, Magnon-phonon interactions in magnetic insulators, *Physical Review B* **99**, 184442 (2019).
  - [17] K. Yamanouchi and K. Shibayama, Propagation and Amplification of Rayleigh Waves and Piezoelectric Leaky Surface Waves in LiNbO<sub>3</sub>, *Journal of Applied Physics* **43**, 856 (1972).
  - [18] R. S. Weis and T. K. Gaylord, Lithium niobate: Summary of physical properties and crystal structure, *Applied Physics A* **37**, 191 (1985).
